# Supplementary material for: Diffutoon-2: Toon Shading with Video Diffusion Models
Source: arXiv:2611.30945 source file (2026-11-23)
Supplement: Supplementary file 1 [file supplementary.tex]

\documentclass[10pt,twocolumn,letterpaper]{article}
\usepackage[pagenumbers]{cvpr}
\input{preamble}
\usepackage[most]{tcolorbox}
\DeclareCaptionType{prompt}[Prompt][List of Prompts]
\captionsetup[prompt]{font=small,labelfont=bf,labelsep=period,justification=raggedright,singlelinecheck=false,hypcap=false}
\tcbset{promptbox/.style={enhanced,colback=black!2!white,
 colframe=black!35,boxrule=0.5pt,arc=1mm,
 left=3mm,right=3mm,top=2mm,bottom=2mm,before skip=3pt,after skip=0pt}}
\newcommand{\promptfile}[3]{%
 \par\addvspace{12pt}\noindent\begin{minipage}{\textwidth}
 \captionof{prompt}{#2}\label{#1}
 \tcbinputlisting{promptbox,listing only,listing file={#3},
 listing options={basicstyle=\ttfamily\small,columns=fullflexible,
 keepspaces=true,breaklines=true,breakatwhitespace=false,
 showstringspaces=false,literate={—}{{\textemdash}}1 {–}{{\textendash}}1}}
 \end{minipage}\par
}

\definecolor{captiongreen}{RGB}{22,112,55}
\definecolor{captionred}{RGB}{176,40,40}
\newcommand{\captionmatch}[1]{\textcolor{captiongreen}{\textbf{#1}}}
\newcommand{\captiondrift}[1]{\textcolor{captionred}{\textbf{#1}}}
\definecolor{cvprblue}{rgb}{0.21,0.49,0.74}
\usepackage[pagebackref,breaklinks,colorlinks,allcolors=cvprblue]{hyperref}
\title{Diffutoon-2: Toon Shading with Video Diffusion Models\\Supplementary Material}
\author{
    Yuze Sun\textsuperscript{1},
    Zhongjie Duan\textsuperscript{1},
    Yingda Chen\textsuperscript{1} and
    Jingjing Chen\textsuperscript{1}\\
    \textsuperscript{1}ModelScope Team, Alibaba Group
}
\begin{document}
\maketitle
\appendix
\input{sec/X_suppl}
{\small\bibliographystyle{ieeenat_fullname}\bibliography{main}}
\end{document}
